# Supplementary material for: Discovery of oxide Li-conducting electrolytes in uncharted chemical space via topology-constrained crystal structure prediction
Source: arXiv:2509.25763 ancillary file (2025-10-01)
Supplement: Supplementary file 1 [file TOPIC-SI.pdf]

## Supplementary Information

### Discovery of oxide Li-conducting electrolytes in uncharted chemical space via topology-constrained crystal structure prediction

Seungwoo Hwang<sup>a</sup>, Jiho Lee<sup>a</sup>, Seungwu Han<sup>a,b</sup>, Youngho Kang<sup>c\*</sup>, and Sungwoo Kang<sup>d,e\*</sup>

<sup>a</sup>*Department of Materials Science and Engineering, Seoul National University, Seoul, 08826, Republic of Korea*

<sup>b</sup>*AI center, Korea Institute of Advanced Study, Seoul, 02455, Republic of Korea*

<sup>c</sup>*Department of Materials Science and Engineering, Incheon National University, Incheon, 22012, Republic of Korea*

<sup>d</sup>*Computational Science Research Center, Korea Institute of Science and Technology (KIST), Seoul, 02792, Republic of Korea*

<sup>e</sup>*Division of Nanoscience and Technology, KIST School, University of Science and Technology (UST), Seoul, 02792, Republic of Korea*

\* Corresponding authors: [youngho84@inu.ac.kr](mailto:youngho84@inu.ac.kr), [sung.w.kang@kist.re.kr](mailto:sung.w.kang@kist.re.kr)

## Supplementary Figures.

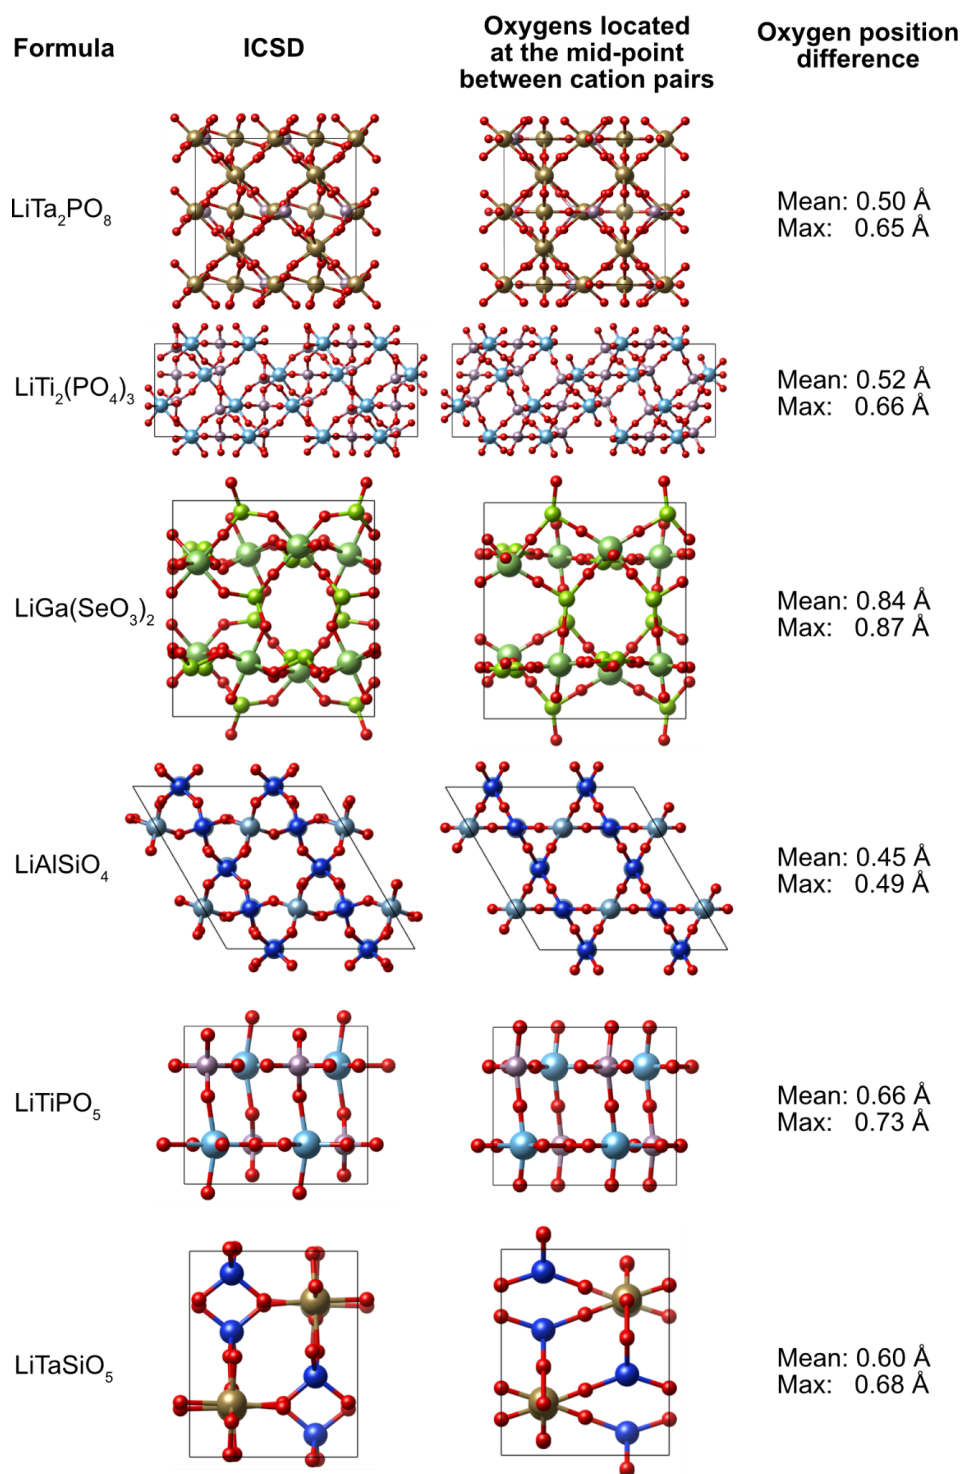

**Fig. S1. Validation of O-atom placement at cation–cation midpoints.** Framework structures are shown for experimentally reported reference compounds (ICSD)<sup>1</sup> and for corresponding models with the same cation sublattice, where O atoms were constrained to the midpoints of cation pairs. The mean and maximum deviations of O-atom positions from the ICSD references are indicated at right. In all cases, O atoms constrained to midpoints remain close to their experimental positions, with no deviation exceeding 1 Å.

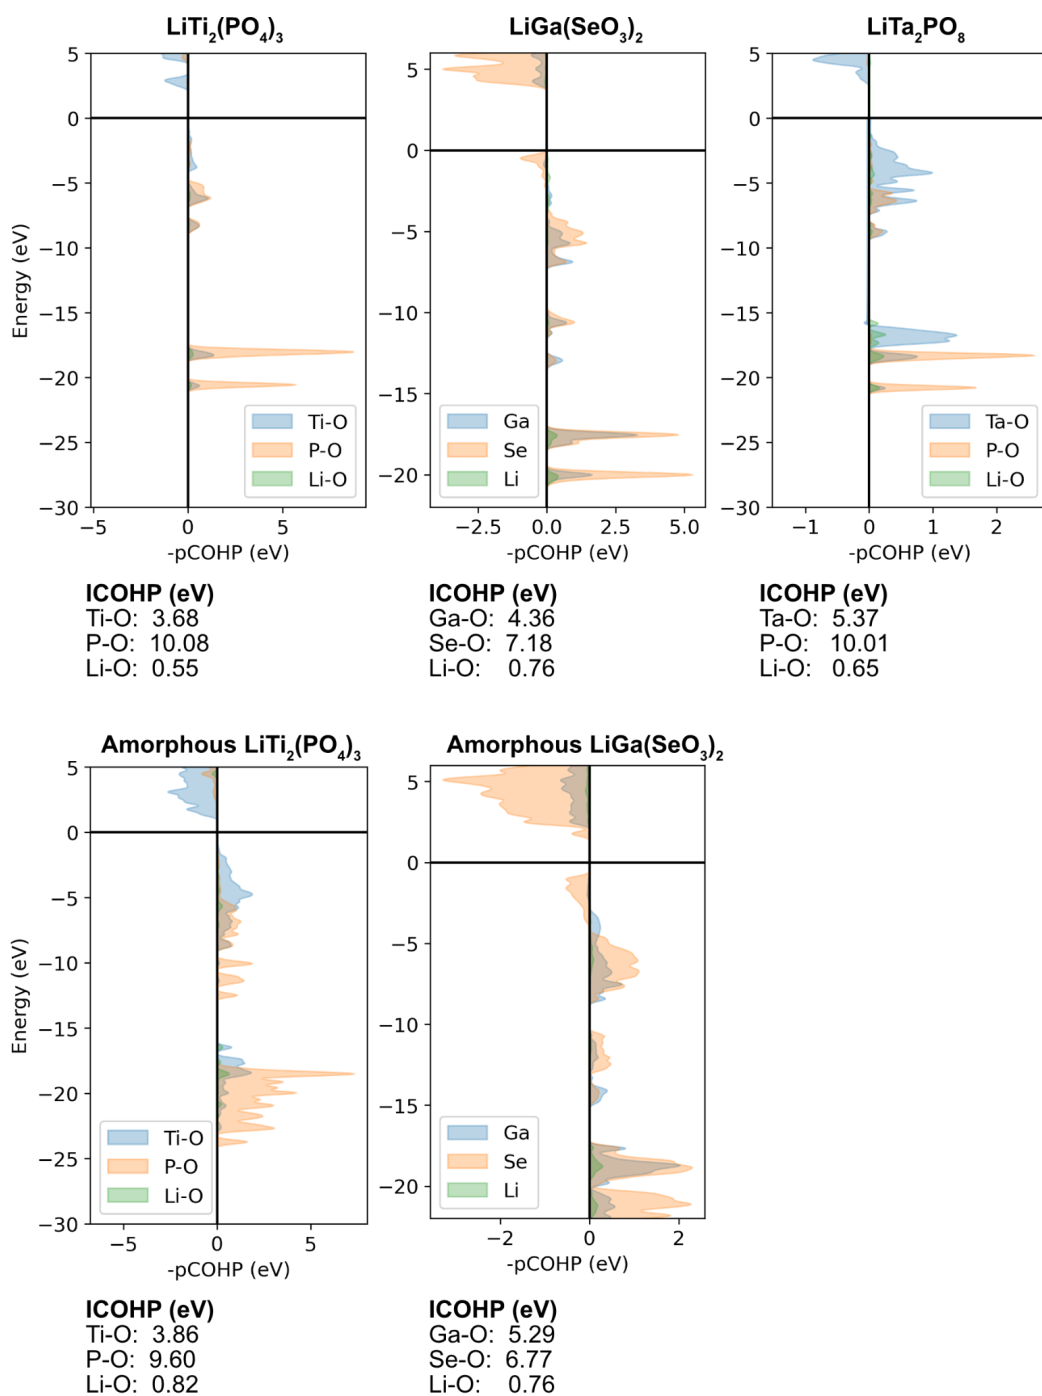

**Fig. S2. Crystal orbital Hamilton population (COHP) analysis<sup>2</sup> of validation systems.** Top panels: COHP plots for crystalline  $\text{LiTi}_2(\text{PO}_4)_3$ ,  $\text{LiGa}(\text{SeO}_3)_2$ , and  $\text{LiTa}_2\text{PO}_8$ , resolved into framework cation–O and Li–O contributions. Bottom panels: corresponding COHP analyses for their melt-quenched amorphous phases. For each case, the integrated COHP (ICOHP) values, reported below the plots, quantify bond strength. Across both crystalline and amorphous systems, Li–O interactions are consistently the weakest compared with framework cation–O bonds, confirming the minor structural role of Li.

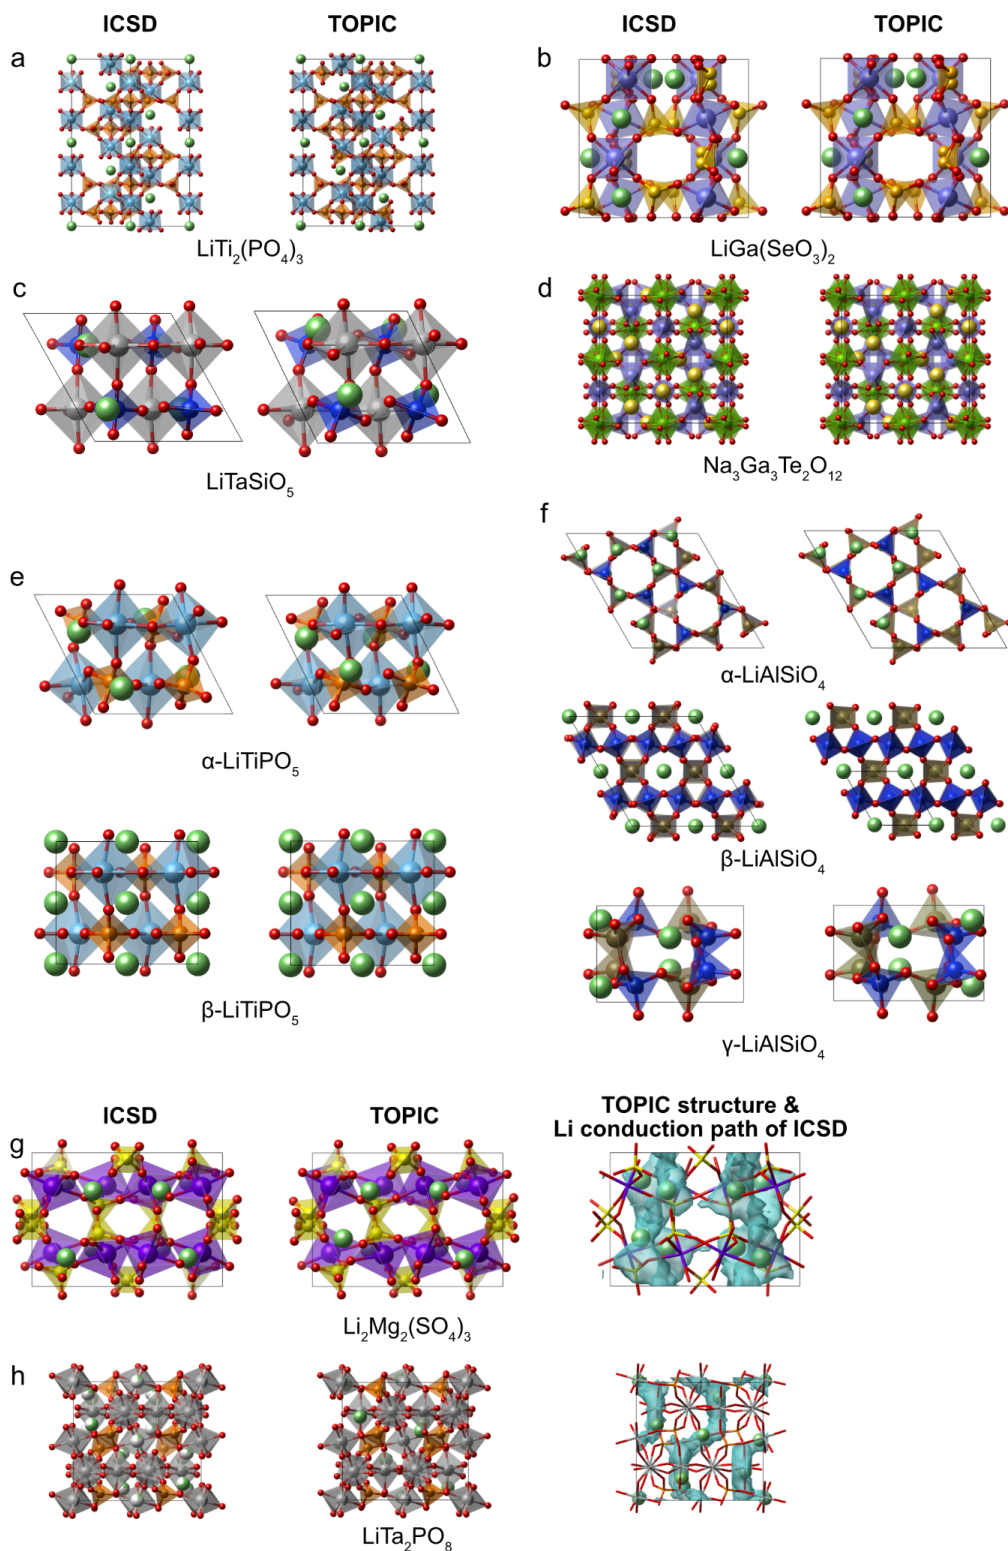

**Fig. S3. Comparison of TOPIC-predicted structures with experimentally reported reference structures.** For each system, the reference (ICSD) structure is shown alongside the corresponding TOPIC prediction. Among ten target compounds with ordered Li sites, TOPIC reproduces six with the correct Li positions ( $\text{LiTi}_2(\text{PO}_4)_3$ ,  $\text{LiGa}(\text{SeO}_3)_2$ ,  $\text{Na}_3\text{Ga}_3\text{Te}_2\text{O}_{12}$ ,  $\beta\text{-LiTiPO}_5$ ,  $\alpha\text{-LiAlSiO}_4$ , and  $\beta\text{-LiAlSiO}_4$ ), while the remaining cases preserve the correct polyhedral connectivity with minor distortions ( $\text{LiTaSiO}_5$ ,  $\alpha\text{-LiTiPO}_5$ , and  $\gamma\text{-LiAlSiO}_4$ ) or deviations in Li sites ( $\text{Li}_2\text{Mg}_2(\text{SO}_4)_3$ ). For (g)  $\text{Li}_2\text{Mg}_2(\text{SO}_4)_3$  and (h)  $\text{LiTa}_2\text{PO}_8$ , Li conduction pathways obtained from molecular dynamics simulations initialized from the ICSD structures are overlaid on the TOPIC-predicted structures, confirming that predicted Li sites fall within established transport channels.

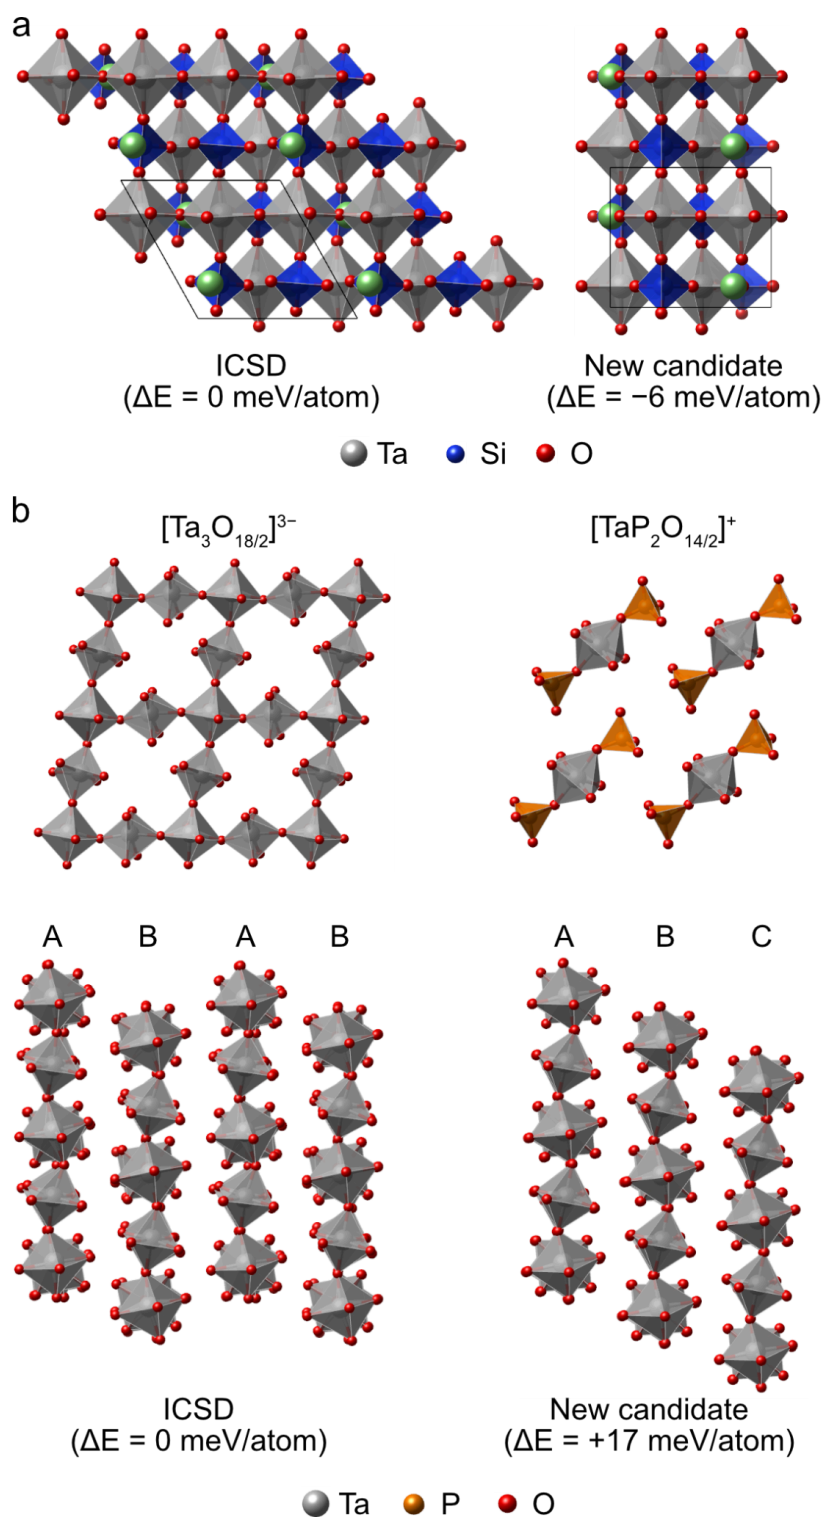

**Fig. S4. Unreported low-energy structures in validation systems predicted by TOPIC.** (a) Comparison between the ICSD reference structure and the TOPIC-identified structure of the  $\text{LiTaSiO}_5$  system. The predicted phase, distinguished by a different stacking sequence, is  $6 \text{ meV atom}^{-1}$  lower in energy than the reported structure. (b) Predicted metastable polymorph of  $\text{LiTa}_2\text{PO}_8$ , lying  $17 \text{ meV atom}^{-1}$  above the reported phase. Top: polyhedral motifs— $[\text{Ta}_3\text{O}_{18/2}]^{3-}$  and  $[\text{TaP}_2\text{O}_{14/2}]^+$ —as described in Ref.<sup>3</sup> for the known structure. Bottom: stacking sequence of the  $[\text{Ta}_3\text{O}_{18/2}]^{3-}$  motif in both the ICSD and TOPIC-predicted structures, together with their relative energies.

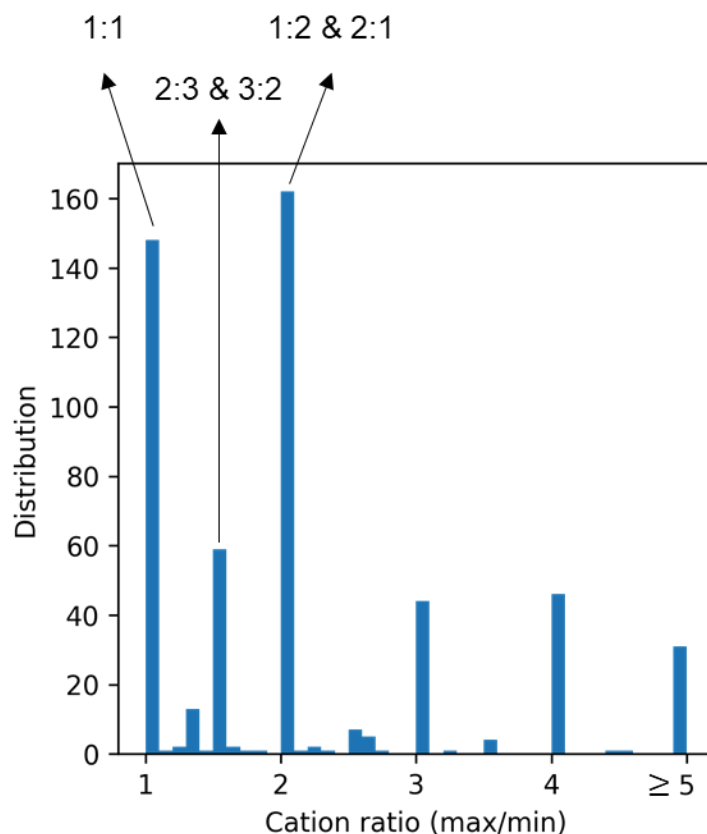

**Fig. S5. Distribution of cation ratios in experimentally reported Li-containing quaternary oxides.** The cation ratio is defined as the maximum number of cations divided by the minimum number of cations in a given composition (excluding Li), based on entries from the Materials Project database.<sup>4</sup> The most frequently observed ratios are 1:1, 2:1 (and its inverse 1:2), and 3:2 (and its inverse 2:3), which are highlighted in the plot. These ratios form the basis for selecting candidate compositions explored in this work.

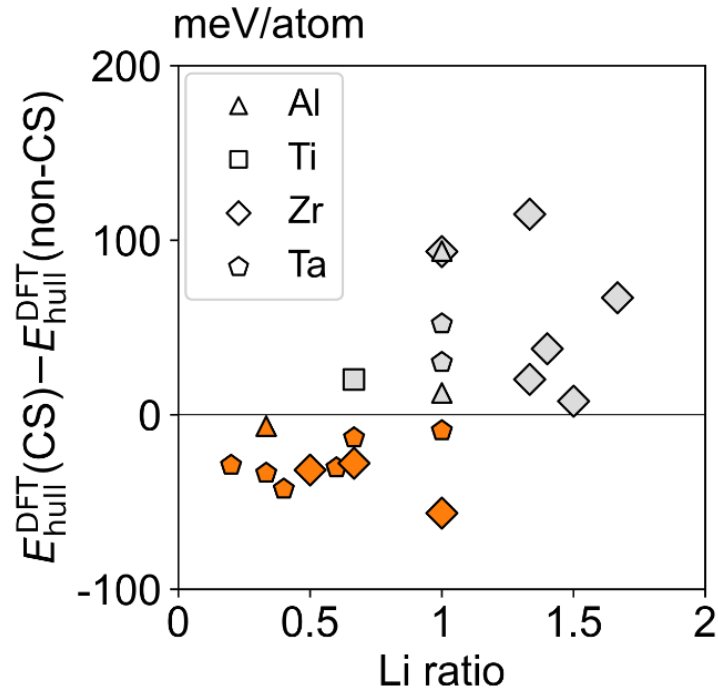

**Fig. S6. Relative stability of CS and non-CS frameworks in SPINNER-generated structures.** Scatter plot of the  $E_{hull}^{DFT}(CS) - E_{hull}^{DFT}(non-CS)$  as a function of Li ratio for each composition. A positive correlation between  $E_{hull}^{DFT}(CS) - E_{hull}^{DFT}(non-CS)$  and Li ratio is maintained, and no stable CS-topology structures are found at Li ratios above 1.0.

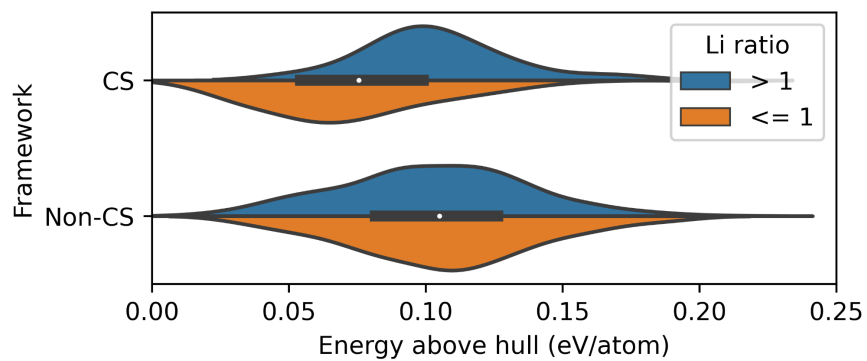

**Fig. S7. Energy-above-hull distributions of CS and non-CS frameworks at low and high Li ratios.** Violin plots show the stability of CS and non-CS structures, grouped by Li ratio ( $\leq 1$  vs.  $> 1$ ). Non-CS frameworks exhibit similar stability distributions across both Li-ratio groups, whereas CS frameworks are more stable at low Li ratios and less stable at high Li ratios.



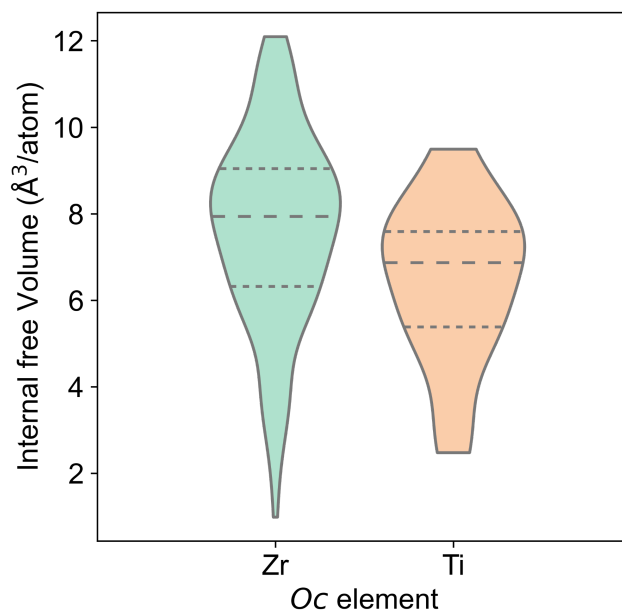

**Fig. S8. Internal free-volume distributions in Zr- and Ti-containing frameworks.** Violin plots show the distributions of internal free volumes for structures where Zr or Ti occupy octahedral sites. The dashed lines mark the quartiles of each distribution. Frameworks with Zr exhibit systematically larger internal free volumes than those with Ti, consistent with the larger ionic radius of  $\text{Zr}^{4+}$  (86 pm) compared to  $\text{Ti}^{4+}$  (75 pm).

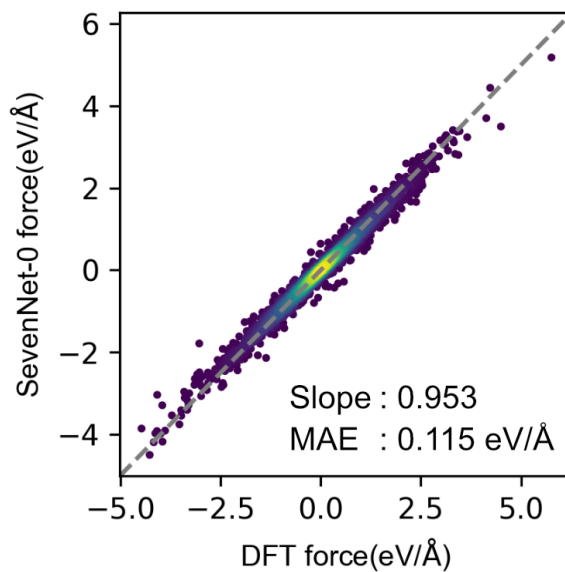

**Fig. S9. Validation of force predictions from SevenNet-0.** Parity plot comparing MLIP (SevenNet-0)<sup>5</sup> and DFT forces from 1000 K molecular dynamics (MD) trajectories of a test structure, Zn-substituted  $\text{LiIn}(\text{IO}_3)_4$  (Materials Project ID: mp-973966), for which systematic force softening was previously reported.<sup>6</sup> The fitted slope (0.953) and mean absolute error ( $\text{MAE} = 0.115 \text{ eV } \text{\AA}^{-1}$ ) indicate close agreement with DFT and show no evidence of systematic softening of the potential energy surface.

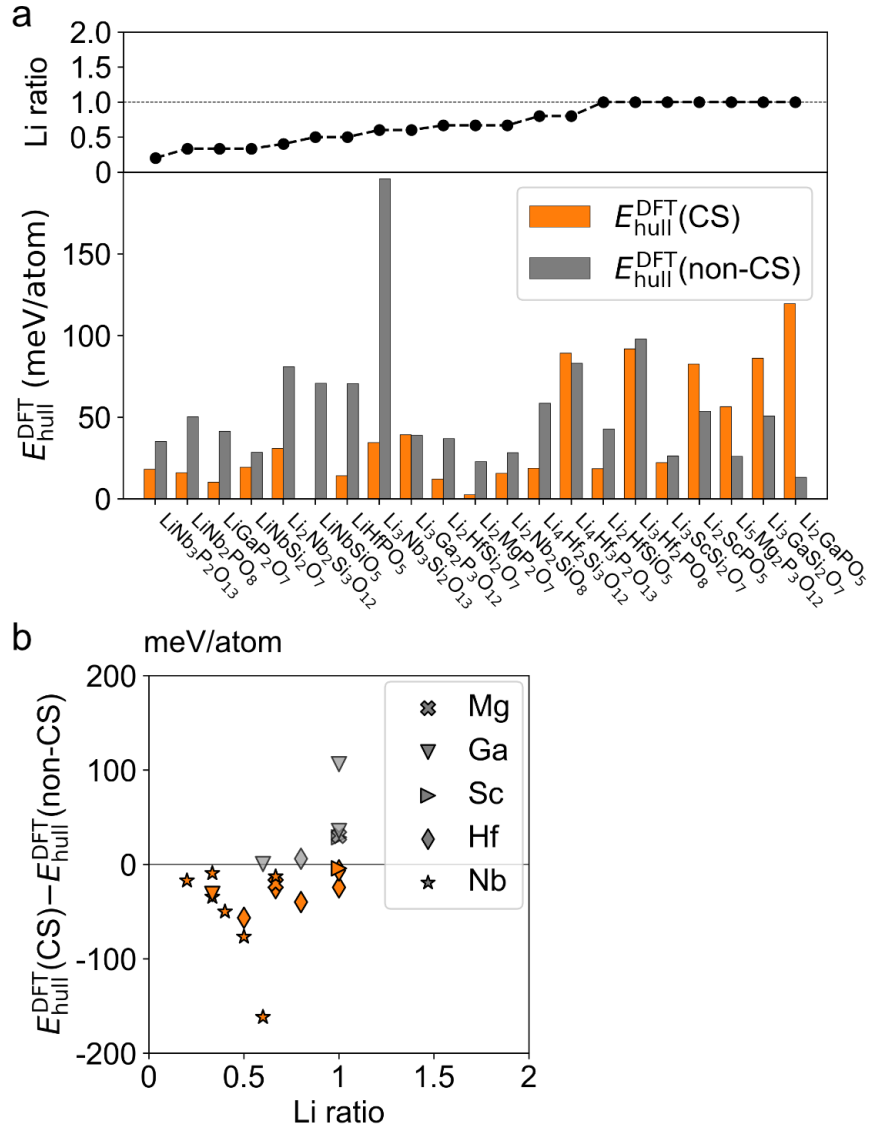

**Fig. S10. Stability of CS and non-CS frameworks as a function of Li ratio.** (a) DFT hull energies of the lowest-energy CS (orange) and non-CS (gray) structures for each composition. Compositions are ordered first by Li ratio and then by the energy difference between CS and non-CS structures within each ratio group. (b) Scatter plot of  $E_{\text{hull}}^{\text{DFT}}(\text{CS}) - E_{\text{hull}}^{\text{DFT}}(\text{non-CS})$  versus Li ratio for each composition.

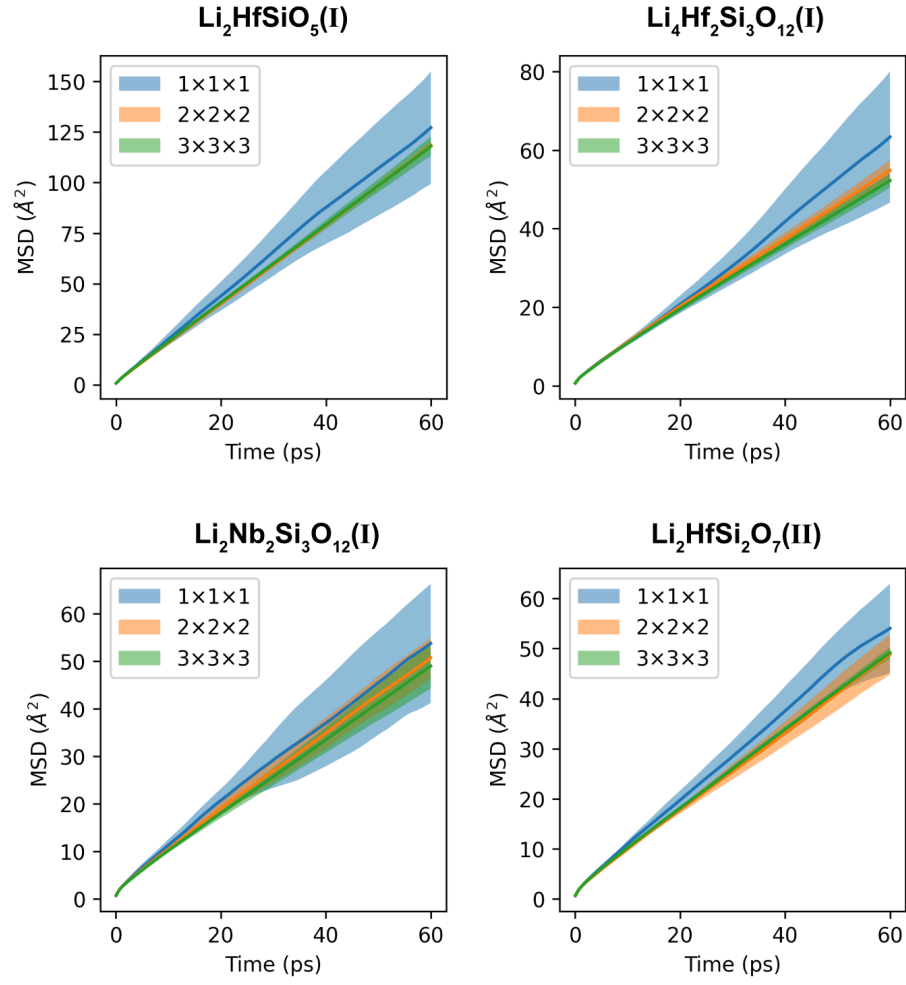

**Fig. S11. Cell-size dependence of computed diffusion.** Mean-squared displacement (MSD) curves from MD simulations at 1000 K using SevenNet-0 are shown for unit cells,  $2 \times 2 \times 2$  supercells, and  $3 \times 3 \times 3$  supercells across representative systems. The results demonstrate negligible finite-size effects in the calculated diffusion coefficients.

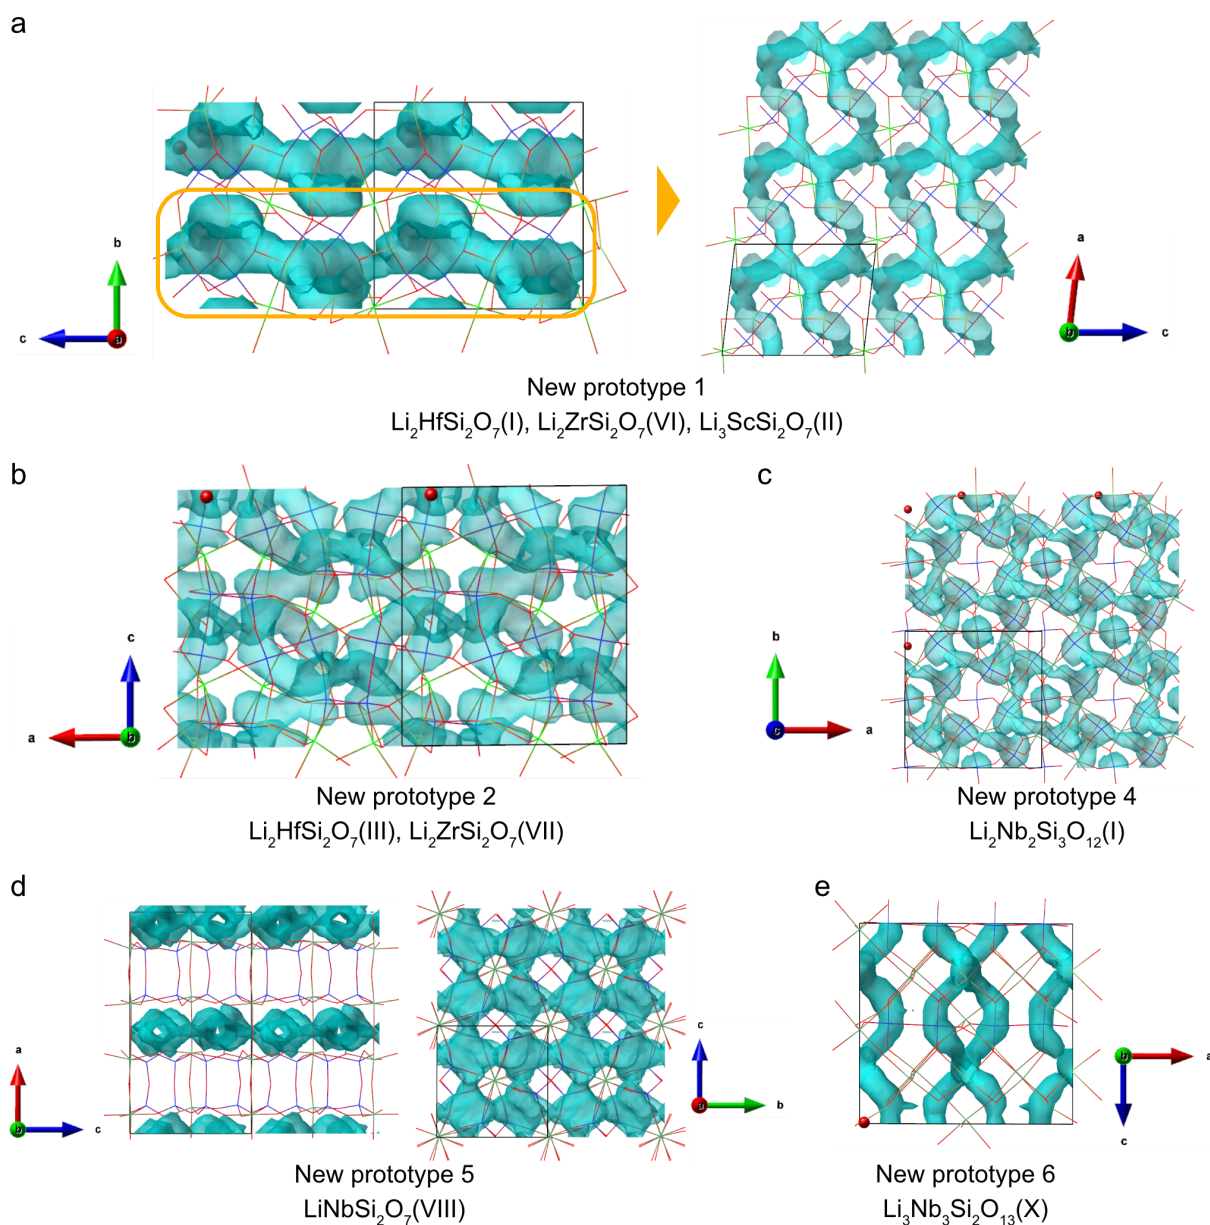

**Fig. S12. Li-ion conduction pathways in candidate oxide solid electrolyte structures.** Isosurfaces of Li probability density from DFT-MD simulations highlight conduction channels in representative candidates with novel frameworks. (a) Quasi two-dimensional pathways in  $\text{Li}_2\text{HfSi}_2\text{O}_7(\text{I})$ ,  $\text{Li}_2\text{ZrSi}_2\text{O}_7(\text{VI})$ , and  $\text{Li}_3\text{ScSi}_2\text{O}_7(\text{II})$ . Left: side view; right: top view (boxed in orange). (b) Three-dimensional pathways in  $\text{Li}_2\text{HfSi}_2\text{O}_7(\text{III})$  and  $\text{Li}_2\text{ZrSi}_2\text{O}_7(\text{VII})$ . (c) Three-dimensional pathways in  $\text{Li}_2\text{Nb}_2\text{Si}_3\text{O}_{12}(\text{I})$ . (d) Quasi two-dimensional pathways in  $\text{LiNbSi}_2\text{O}_7(\text{VIII})$ . Left: side view; right: top view. (e) Quasi one-dimensional pathways in  $\text{Li}_3\text{Nb}_3\text{Si}_2\text{O}_{13}(\text{X})$ .

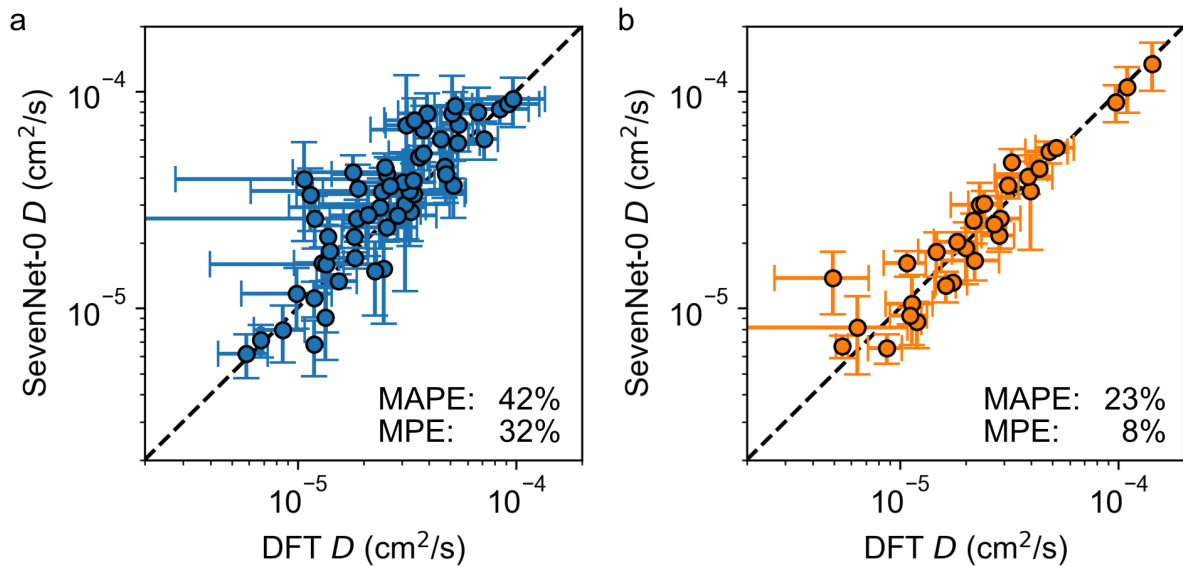

**Fig. S13. Comparison of diffusion coefficients predicted by SevenNet-0 and DFT.** (a) Parity plot for materials with novel prototype structures. (b) Parity plot for materials with known prototype structures (NASICON-,  $\text{LiTaSiO}_5$ -, and  $\beta\text{-LiTiPO}_5$ -type). Error bars represent the standard deviation from independent MD runs. SevenNet-0 often overestimates diffusion in novel prototypes but shows close agreement with DFT for known structure types.

## Supplementary Table.

**Table S1. Ionic radii and coordination numbers (CN) used in this study.** Shannon ionic radii<sup>7</sup> are listed along with the corresponding coordination numbers. The cation-to-oxygen radius ratio ( $r_C/r_O$ ) is also presented. According to Pauling's rule,<sup>8</sup>  $r_C/r_O$  values of 0.225–0.414 favor tetrahedral coordination (CN = 4), while values of 0.414–0.645 favor octahedral coordination (CN = 6).

| Ion                    | Coordination number | Ionic radius (pm) | $r_C/r_O$ |
|------------------------|---------------------|-------------------|-----------|
| <b>Mg<sup>2+</sup></b> | 6                   | 86                | 0.683     |
| <b>Al<sup>3+</sup></b> | 4                   | 53                | 0.421     |
|                        | 6                   | 67.5              | 0.536     |
| <b>Si<sup>4+</sup></b> | 4                   | 40                | 0.317     |
| <b>P<sup>5+</sup></b>  | 4                   | 31                | 0.246     |
| <b>S<sup>6+</sup></b>  | 4                   | 26                | 0.206     |
| <b>Sc<sup>3+</sup></b> | 6                   | 88.5              | 0.702     |
| <b>Ti<sup>4+</sup></b> | 6                   | 75                | 0.595     |

| Ion                    | Coordination number | Ionic radius (pm) | $r_C/r_O$ |
|------------------------|---------------------|-------------------|-----------|
| <b>Ga<sup>3+</sup></b> | 4                   | 61                | 0.484     |
|                        | 6                   | 76                | 0.603     |
| <b>Se<sup>3+</sup></b> | 3                   | 42                | 0.333     |
| <b>Zr<sup>4+</sup></b> | 6                   | 86                | 0.683     |
| <b>Nb<sup>5+</sup></b> | 6                   | 78                | 0.619     |
| <b>Te<sup>6+</sup></b> | 6                   | 70                | 0.556     |
| <b>Hf<sup>4+</sup></b> | 6                   | 85                | 0.675     |
| <b>Ta<sup>5+</sup></b> | 6                   | 78                | 0.619     |

**Table S2. Comparison of activation energies and ionic conductivities obtained from DFT and SevenNet-0.** Activation energies ( $E_a$ ) and room-temperature ionic conductivities ( $\sigma_{300K}$ ) are listed for pristine LiGa(SeO<sub>3</sub>)<sub>2</sub> and doped systems (Ga-doped LiTiPO<sub>5</sub> and P-doped Li<sub>2</sub>Mg<sub>2</sub>(SO<sub>4</sub>)<sub>3</sub>). SevenNet-0 also reproduces the activation energy of LiTa<sub>2</sub>PO<sub>8</sub>, which was not included in its training set. The results demonstrate that SevenNet-0 predicts both activation energies and conductivities with reasonable accuracy compared to DFT.

| System                                                                  | Reference         | $E_a$ (DFT)   | $E_a$ (SevenNet-0) | $\sigma_{300K}$ (DFT) | $\sigma_{300K}$ (SevenNet-0) |
|-------------------------------------------------------------------------|-------------------|---------------|--------------------|-----------------------|------------------------------|
| LiGa(SeO <sub>3</sub> ) <sub>2</sub>                                    | Ref <sup>9</sup>  | 0.320 ± 0.070 | 0.356 ± 0.058      | 0.212 (0.013, 3.57)   | 0.057                        |
| Ga-doped LiTiPO <sub>5</sub>                                            | Ref <sup>9</sup>  | 0.212 ± 0.071 | 0.267 ± 0.016      | 1.70 (0.098, 29.7)    | 0.385                        |
| P-doped Li <sub>2</sub> Mg <sub>2</sub> (SO <sub>4</sub> ) <sub>3</sub> | Ref <sup>9</sup>  | 0.232 ± 0.073 | 0.227 ± 0.058      | 2.74 (0.145, 52.0)    | 3.54                         |
| LiTa <sub>2</sub> PO <sub>8</sub>                                       | Ref <sup>10</sup> | 0.16          | 0.160 ± 0.013      | 35.3                  | 28.85                        |



**Table S3. DFT hull energies of CS and non-CS frameworks for 45 target quaternary compositions.** For each formula, the Li ratio,  $E_{hull}^{DFT}$  (CS), and  $E_{hull}^{DFT}$  (non-CS) (in meV atom<sup>-1</sup>) are listed. The comparison highlights the relative stability of CS versus non-CS frameworks across different Li ratios, supporting the robustness of the Li-ratio descriptor.

| Formula                                                         | Li ratio | $E_{hull}^{DFT}$ (CS) | $E_{hull}^{DFT}$ (non-CS) | Formula                                                         | Li ratio | $E_{hull}^{DFT}$ (CS) | $E_{hull}^{DFT}$ (non-CS) |
|-----------------------------------------------------------------|----------|-----------------------|---------------------------|-----------------------------------------------------------------|----------|-----------------------|---------------------------|
| LiTa <sub>3</sub> P <sub>2</sub> O <sub>13</sub>                | 0.200    | <b><u>19.2</u></b>    | 88.8                      | Li <sub>4</sub> Zr <sub>2</sub> Si <sub>3</sub> O <sub>12</sub> | 0.800    | <b><u>34.1</u></b>    | 75.2                      |
| LiNb <sub>3</sub> P <sub>2</sub> O <sub>13</sub>                | 0.200    | <b><u>18.1</u></b>    | 35.2                      | Li <sub>4</sub> Hf <sub>2</sub> Si <sub>3</sub> O <sub>12</sub> | 0.800    | <b><u>21.3</u></b>    | 58.6                      |
| LiNb <sub>2</sub> PO <sub>8</sub>                               | 0.333    | <b><u>16.1</u></b>    | 50.3                      | Li <sub>4</sub> Ti <sub>2</sub> Si <sub>3</sub> O <sub>12</sub> | 0.800    | 61.2                  | <b><u>57.1</u></b>        |
| LiTaSi <sub>2</sub> O <sub>7</sub>                              | 0.333    | <b><u>16.0</u></b>    | 49.4                      | Li <sub>4</sub> Hf <sub>3</sub> P <sub>2</sub> O <sub>13</sub>  | 0.800    | 89.3                  | <b><u>83.1</u></b>        |
| LiGaP <sub>2</sub> O <sub>7</sub>                               | 0.333    | <b><u>10.3</u></b>    | 41.4                      | Li <sub>4</sub> Zr <sub>3</sub> P <sub>2</sub> O <sub>13</sub>  | 0.800    | 100.7                 | <b><u>93.8</u></b>        |
| LiAlP <sub>2</sub> O <sub>7</sub>                               | 0.333    | <b><u>2.1</u></b>     | 27.1                      | Li <sub>4</sub> Ti <sub>3</sub> P <sub>2</sub> O <sub>13</sub>  | 0.800    | 133.5                 | <b><u>79.2</u></b>        |
| LiNbSi <sub>2</sub> O <sub>7</sub>                              | 0.333    | <b><u>19.4</u></b>    | 28.5                      | Li <sub>2</sub> ZrSiO <sub>5</sub>                              | 1.000    | <b><u>26.9</u></b>    | 86.6                      |
| Li <sub>2</sub> Ta <sub>2</sub> Si <sub>3</sub> O <sub>12</sub> | 0.400    | <b><u>10.9</u></b>    | 90.7                      | Li <sub>3</sub> TaAl <sub>2</sub> O <sub>7</sub>                | 1.000    | <b><u>17.8</u></b>    | 52.9                      |
| Li <sub>2</sub> Nb <sub>2</sub> Si <sub>3</sub> O <sub>12</sub> | 0.400    | <b><u>30.9</u></b>    | 80.9                      | Li <sub>5</sub> Ta <sub>3</sub> Al <sub>2</sub> O <sub>13</sub> | 1.000    | <b><u>58.1</u></b>    | 87.0                      |
| LiNbSiO <sub>5</sub>                                            | 0.500    | <b><u>0</u></b>       | 76.7                      | Li <sub>2</sub> HfSiO <sub>5</sub>                              | 1.000    | <b><u>18.6</u></b>    | 42.8                      |
| LiHfPO <sub>5</sub>                                             | 0.500    | <b><u>14.2</u></b>    | 70.7                      | Li <sub>2</sub> TaAlO <sub>5</sub>                              | 1.000    | <b><u>17.1</u></b>    | 34.0                      |
| LiZrPO <sub>5</sub>                                             | 0.500    | <b><u>26.9</u></b>    | 58.5                      | Li <sub>3</sub> Ta <sub>2</sub> AlO <sub>8</sub>                | 1.000    | <b><u>15.2</u></b>    | 26.6                      |
| Li <sub>3</sub> Nb <sub>3</sub> Si <sub>2</sub> O <sub>13</sub> | 0.600    | <b><u>34.5</u></b>    | 196.1                     | Li <sub>3</sub> Hf <sub>2</sub> PO <sub>8</sub>                 | 1.000    | <b><u>91.8</u></b>    | 97.9                      |
| Li <sub>3</sub> Ta <sub>3</sub> Si <sub>2</sub> O <sub>13</sub> | 0.600    | <b><u>35.3</u></b>    | 86.2                      | Li <sub>3</sub> ScSi <sub>2</sub> O <sub>7</sub>                | 1.000    | <b><u>22.3</u></b>    | 26.3                      |
| Li <sub>3</sub> Al <sub>2</sub> P <sub>3</sub> O <sub>12</sub>  | 0.600    | <b><u>43.2</u></b>    | 60.6                      | Li <sub>3</sub> AlSi <sub>2</sub> O <sub>7</sub>                | 1.000    | 57.2                  | <b><u>44.7</u></b>        |
| Li <sub>3</sub> Ga <sub>2</sub> P <sub>3</sub> O <sub>12</sub>  | 0.600    | 39.3                  | <b><u>38.9</u></b>        | Li <sub>5</sub> Ta <sub>2</sub> Al <sub>3</sub> O <sub>12</sub> | 1.000    | 71.2                  | <b><u>56.4</u></b>        |
| Li <sub>2</sub> ZrSi <sub>2</sub> O <sub>7</sub>                | 0.667    | <b><u>25.9</u></b>    | 58.8                      | Li <sub>3</sub> Zr <sub>2</sub> PO <sub>8</sub>                 | 1.000    | 135.3                 | <b><u>114.5</u></b>       |
| Li <sub>2</sub> HfSi <sub>2</sub> O <sub>7</sub>                | 0.667    | <b><u>12.1</u></b>    | 37.0                      | Li <sub>2</sub> ScPO <sub>5</sub>                               | 1.000    | 82.5                  | <b><u>53.6</u></b>        |
| Li <sub>2</sub> MgP <sub>2</sub> O <sub>7</sub>                 | 0.667    | <b><u>2.6</u></b>     | 22.8                      | Li <sub>5</sub> Mg <sub>2</sub> P <sub>3</sub> O <sub>12</sub>  | 1.000    | 56.6                  | <b><u>26.1</u></b>        |
| Li <sub>2</sub> Ta <sub>2</sub> SiO <sub>8</sub>                | 0.667    | <b><u>17.9</u></b>    | 32.8                      | Li <sub>3</sub> GaSi <sub>2</sub> O <sub>7</sub>                | 1.000    | 86.1                  | <b><u>50.7</u></b>        |
| Li <sub>2</sub> Nb <sub>2</sub> SiO <sub>8</sub>                | 0.667    | <b><u>15.6</u></b>    | 28.3                      | Li <sub>2</sub> AlPO <sub>5</sub>                               | 1.000    | 122.6                 | <b><u>28.7</u></b>        |
| Li <sub>2</sub> TiSi <sub>2</sub> O <sub>7</sub>                | 0.667    | 45.0                  | <b><u>29.4</u></b>        | Li <sub>2</sub> GaPO <sub>5</sub>                               | 1.000    | 119.5                 | <b><u>13.2</u></b>        |
|                                                                 |          |                       |                           | Li <sub>3</sub> Ti <sub>2</sub> PO <sub>8</sub>                 | 1.000    | -                     | <b><u>69.8</u></b>        |

**Table S4 | Frequently occurring frameworks identified in the comprehensive screening.** Listed are representative chemical formulas and their activation energies ( $E_a$ ), grouped by framework type and Li ratio. Experimental  $E_a$  values for  $\text{LiTi}_2(\text{PO}_4)_3$  and  $\text{LiTiPO}_5$  are taken from the literature.<sup>11–15</sup>

| Framework type                    | Li ratio | Formula                                          | $E_a$ (eV) | Reference             |
|-----------------------------------|----------|--------------------------------------------------|------------|-----------------------|
| NASICON-type                      | 0.2      | $\text{LiTi}_2(\text{PO}_4)_3$                   | 0.30~0.46  | Ref. <sup>11–14</sup> |
|                                   | 0.4      | $\text{Li}_2\text{Nb}_2\text{Si}_3\text{O}_{12}$ | 0.267      | -                     |
|                                   |          | $\text{Li}_2\text{Ta}_2\text{Si}_3\text{O}_{12}$ | 0.306      | -                     |
|                                   | 0.8      | $\text{Li}_4\text{Hf}_2\text{Si}_3\text{O}_{12}$ | 0.183      | -                     |
|                                   |          | $\text{Li}_4\text{Zr}_2\text{Si}_3\text{O}_{12}$ | 0.270      | -                     |
| $\beta$ - $\text{LiTiPO}_5$ -type | 0.5      | $\text{LiTiPO}_5$                                | 1.00       | Ref. <sup>15</sup>    |
|                                   | 1.0      | $\text{Li}_2\text{HfSiO}_5$                      | 0.375      | -                     |
| New prototype 1                   | 0.667    | $\text{Li}_2\text{ZrSi}_2\text{O}_7$             | 0.277      | -                     |
|                                   |          | $\text{Li}_2\text{HfSi}_2\text{O}_7$             | 0.319      | -                     |
|                                   | 1.0      | $\text{Li}_3\text{ScSi}_2\text{O}_7$             | 0.236      | -                     |
| New prototype 3                   | 0.333    | $\text{LiTa}_2\text{PO}_8$                       | 0.125      | -                     |
|                                   | 0.667    | $\text{Li}_2\text{Ta}_2\text{SiO}_8$             | 0.562      | -                     |
|                                   | 1.0      | $\text{Li}_3\text{Ta}_2\text{AlO}_8$             | 0.242      | -                     |

**Table S5 Continuous Symmetry Measure (CSM) analysis<sup>9,16</sup> of Li environments.** CSM values are reported for Li ions in octahedral and tetrahedral sites across  $\beta$ -LiTiPO<sub>5</sub>-, NASICON-, and new prototype 1 frameworks. Larger CSM values indicate greater deviations from ideal site symmetry, reflecting the structural distortions induced by Li stuffing.

| Prototype                         | Formula                                                         | Octahedral site CSM | Tetrahedral site CSM |
|-----------------------------------|-----------------------------------------------------------------|---------------------|----------------------|
| $\beta$ -LiTiPO <sub>5</sub> type | LiTiPO <sub>5</sub>                                             | 2.2                 | -                    |
|                                   | Li <sub>2</sub> HfSiO <sub>5</sub>                              | -                   | 5.4, 8.2             |
| NASICON type                      | LiTi <sub>2</sub> P <sub>3</sub> O <sub>12</sub>                | 5.0                 | -                    |
|                                   | Li <sub>2</sub> Ta <sub>2</sub> Si <sub>3</sub> O <sub>12</sub> | 23.0 ~ 24           | 10.6 ~ 15.1          |
|                                   | Li <sub>2</sub> Nb <sub>2</sub> Si <sub>3</sub> O <sub>12</sub> | 24.1                | 13.7                 |
|                                   | Li <sub>4</sub> Hf <sub>2</sub> Si <sub>3</sub> O <sub>12</sub> | 19.4                | 1.8 ~ 23.3           |
|                                   | Li <sub>4</sub> Zr <sub>2</sub> Si <sub>3</sub> O <sub>12</sub> | 27.5                | 1.4 ~ 3.1            |
|                                   | Li <sub>2</sub> HfSi <sub>2</sub> O <sub>7</sub>                | -                   | 1.8, 8.7             |
| New prototype 1                   | Li <sub>2</sub> ZrSi <sub>2</sub> O <sub>7</sub>                | -                   | 1.5, 8.6             |
|                                   | Li <sub>3</sub> ScSi <sub>2</sub> O <sub>7</sub>                | 11.1                | 1.6 ~ 30.0           |

## References.

- 1 G. Bergerhoff, R. Hundt, R. Sievers and I. D. Brown, *J. Chem. Inf. Comput. Sci.*, 1983, **23**, 66–69.
- 2 V. L. Deringer, A. L. Tchougréeff and R. Dronskowski, *J. Phys. Chem. A*, 2011, **115**, 5461–5466.
- 3 J. Kim, J. Kim, M. Avdeev, H. Yun and S.-J. Kim, *J. Mater. Chem. A*, 2018, **6**, 22478–22482.
- 4 A. Jain, S. P. Ong, G. Hautier, W. Chen, W. D. Richards, S. Dacek, S. Cholia, D. Gunter, D. Skinner, G. Ceder and K. A. Persson, *Apl Mater.*, 2013, **1**, 011002.
- 5 Y. Park, J. Kim, S. Hwang and S. Han, *J. Chem. theory Comput.*, 2024, **20**, 4857–4868.
- 6 B. Deng, Y. Choi, P. Zhong, J. Riebesell, S. Anand, Z. Li, K. Jun, K. A. Persson and G. Ceder, *npj Comput. Mater.*, 2025, **11**, 9.
- 7 R. D. Shannon, *Acta Crystallogr. Sect. A*, 1976, **32**, 751–767.
- 8 L. Pauling, *J. Am. Chem. Soc.*, 1929, **51**, 1010–1026.
- 9 K. Jun, Y. Sun, Y. Xiao, Y. Zeng, R. Kim, H. Kim, L. J. Miara, D. Im, Y. Wang and G. Ceder, *Nat. Mater.*, 2022, **21**, 924–931.
- 10 F. Hussain, P. Li and Z. Li, *J. Phys. Chem. C*, 2019, **123**, 19282–19287.
- 11 Y. Luo, X. Liu, C. Wen, T. Ning, X. Jiang and A. Lu, *Appl. Phys. A*, 2023, **129**, 518.
- 12 K. Takada, M. Tansho, I. Yanase, T. Inada, A. Kajiyama, M. Kouguchi, S. Kondo and M. Watanabe, *Solid State Ion.*, 2001, **139**, 241–247.
- 13 K. Arbi, M. A. París and J. Sanz, *J. Phys. Chem. B*, 2006, **110**, 6454–6457.
- 14 H. Aono, E. Sugimoto, Y. Sadaoka, N. Imanaka and G. Adachi, *Solid State Ion.*, 1991, **47**, 257–264.
- 15 A. Robertson, J. G. Fletcher, J. M. S. Skakle and A. R. West, *J. Solid State Chem.*, 1994, **109**, 53–59.
- 16 D. D. Stefano, A. Miglio, K. Robeyns, Y. Filinchuk, M. Lechartier, A. Senyshyn, H. Ishida, S. Spannenberger, D. Prutsch, S. Lunghammer, D. Rettenwander, M. Wilkening, B. Roling, Y. Kato and G. Hautier, *Chem*, 2019, **5**, 2450–2460.
